# Supplementary material for: Electron transfer across a thermal gradient
Source: arXiv:1607.07010 ancillary file (2016-07-24)
Supplement: Supplementary file 1 [file Craven_Nitzan_Supporting_Information.pdf]

# Supporting Information for "Electron transfer across a thermal gradient"

Galen T. Craven[1] and Abraham Nitzan[1, 2]

[1]*Department of Chemistry, University of Pennsylvania, Philadelphia, PA 19104, USA*

[2]*School of Chemistry, Tel Aviv University, Tel Aviv 69978, Israel*

## I. DERIVATION OF THE NORMAL VELOCITY AT THE CROSSING LINE

In the rate expression given by Eq. (6), the frequency of activated events is proportional to the expectation value of the velocity normal to the transition state. For bithermal electron transfer (ET), the set of transition state structures is composed of equienergetic points between the $E_a$ and $E_b$ surfaces which are elements of the crossing line (CL). A unit normal vector to the CL is

$$\begin{aligned} \hat{\mathbf{u}}_{\rm n} &= (n_1, n_2) \\ &= \left(-\frac{1}{|\nabla g|}, \frac{s}{|\nabla g|}\right) \\ &= n_1 \hat{\mathbf{e}}_1 + n_2 \hat{\mathbf{e}}_2, \end{aligned} \tag{S1}$$

and a unit tangent vector is

$$\begin{aligned} \hat{\mathbf{u}}_{\rm t} &= (n_2, -n_1) \\ &= \left(\frac{s}{|\nabla g|}, \frac{1}{|\nabla g|}\right) \\ &= n_2 \hat{\mathbf{e}}_1 - n_1 \hat{\mathbf{e}}_2, \end{aligned} \tag{S2}$$

where $g(x_1, x_2) = x_1 - s x_2 - c$ is a function that defines the crossing constraint $g(x_1, x_2) = 0$. The slope $s$ is the coefficient in front of $\alpha$ in Eq. (21) and intercept $c$ represents the second term in the r.h.s. of Eq. (21). The constant $|\nabla g| = \sqrt{1+s^2}$ is the magnitude of the gradient of the CL. The velocity vector

$$\dot{\mathbf{x}} = \dot{x}_1 \hat{\mathbf{e}}_1 + \dot{x}_2 \hat{\mathbf{e}}_2 \tag{S3}$$

has a scalar component in the direction of the normal [102],

$$\dot{x}_{\rm n}(\dot{x}_1, \dot{x}_2) = \dot{\mathbf{x}} \cdot \hat{\mathbf{u}}_{\rm n} = \dot{x}_1 n_1 + \dot{x}_2 n_2, \tag{S4}$$

and a scalar component in the direction of the tangent,

$$\dot{x}_{\rm t}(\dot{x}_1, \dot{x}_2) = \dot{\mathbf{x}} \cdot \hat{\mathbf{u}}_{\rm t} = \dot{x}_1 n_2 - \dot{x}_2 n_1. \tag{S5}$$

We are interested calculating the expectation value of the normal component,

$$\langle \dot{x}_{\rm n} \rangle = \frac{\displaystyle\iint_{\mathcal{C}} \dot{x}_{\rm n}(\dot{x}_1, \dot{x}_2)\, e^{-\beta_1\left(\frac{1}{2} m_1 \dot{x}_1^2\right)} e^{-\beta_2\left(\frac{1}{2} m_2 \dot{x}_2^2\right)}\, d\dot{x}_1\, d\dot{x}_2}{\displaystyle\iint_{\mathcal{C}} e^{-\beta_1\left(\frac{1}{2} m_1 \dot{x}_1^2\right)} e^{-\beta_2\left(\frac{1}{2} m_2 \dot{x}_2^2\right)}\, d\dot{x}_1\, d\dot{x}_2} \tag{S6}$$

where $\mathcal{C}$ is a domain of integration such that we only include the positive values of $\dot{x}_{\rm n}$. In order satisfy this constraint we will transform from $\dot{x}_1 \times \dot{x}_2$ space into a coordinate system with basis in the normal and tangential directions.

The normal and tangential velocity components can be defined through

$$\begin{pmatrix} \dot{x}_{\rm n} \\ \dot{x}_{\rm t} \end{pmatrix} = \mathbf{M} \begin{pmatrix} \dot{x}_1 \\ \dot{x}_2 \end{pmatrix}, \tag{S7}$$

with

$$\mathbf{M} = \begin{pmatrix} n_1 & n_2 \\ n_2 & -n_1 \end{pmatrix}, \tag{S8}$$

which allows the components $\dot{x}_1$ and $\dot{x}_2$ to be expressed as

$$\begin{pmatrix} \dot{x}_1 \\ \dot{x}_2 \end{pmatrix} = \mathbf{M}^{-1} \begin{pmatrix} \dot{x}_{\rm n} \\ \dot{x}_{\rm t} \end{pmatrix}, \tag{S9}$$

with

$$\det \mathbf{M} = |\mathbf{M}| = -\left(n_1^2 + n_2^2\right). \tag{S10}$$

and

$$\mathbf{M}^{-1} = \frac{1}{|\mathbf{M}|} \begin{pmatrix} -n_1 & -n_2 \\ -n_2 & n_1 \end{pmatrix}. \tag{S11}$$

Expanding Eq. (S9) yields,

$$\dot{x}_1(\dot{x}_{\rm n}, \dot{x}_{\rm t}) = \frac{1}{|\mathbf{M}|}\left(-n_1 \dot{x}_{\rm n} - n_2 \dot{x}_{\rm t}\right), \tag{S12}$$

$$\dot{x}_2(\dot{x}_{\rm n}, \dot{x}_{\rm t}) = \frac{1}{|\mathbf{M}|}\left(-n_2 \dot{x}_{\rm n} + n_1 \dot{x}_{\rm t}\right). \tag{S13}$$

which express the respective original coordinate in terms of the normal and tangential components. In the diagonal (normal-tangential) coordinate system, the expectation value of the normal velocity in the positive direction is

$$\langle v_\perp \rangle = \langle \dot{x}_\mathrm{n} \rangle = \frac{\int_0^\infty \int_{-\infty}^\infty \dot{x}_\mathrm{n} \exp\left[-\beta_1 \left(\frac{1}{2} m_1 \left[\dot{x}_1(\dot{x}_\mathrm{n}, \dot{x}_\mathrm{t})\right]^2\right)\right] \exp\left[-\beta_2 \left(\frac{1}{2} m_2 \left[\dot{x}_2(\dot{x}_\mathrm{n}, \dot{x}_\mathrm{t})\right]^2\right)\right] d\dot{x}_\mathrm{t}\, d\dot{x}_\mathrm{n}}{\int_0^\infty \int_{-\infty}^\infty \exp\left[-\beta_1 \left(\frac{1}{2} m_1 \left[\dot{x}_1(\dot{x}_\mathrm{n}, \dot{x}_\mathrm{t})\right]^2\right)\right] \exp\left[-\beta_2 \left(\frac{1}{2} m_2 \left[\dot{x}_2(\dot{x}_\mathrm{n}, \dot{x}_\mathrm{t})\right]^2\right)\right] d\dot{x}_\mathrm{t}\, d\dot{x}_\mathrm{n}}, \tag{S14}$$

which upon evaluation yields

$$\langle \dot{x}_\mathrm{n} \rangle = \sqrt{\frac{2}{\pi}\left(\frac{m_2\beta_2 n_1^2 + m_1\beta_1 n_2^2}{m_1\beta_1 m_2\beta_2}\right)}. \tag{S15}$$

At the unithermal ($\beta_1 = \beta_2 = \beta$) - equimass ($m_1 = m_2 = m$) limit, Eq. (S15) reduces to the expected form

$$\langle \dot{x}_\mathrm{n} \rangle = \sqrt{\frac{2}{\pi m \beta}}, \tag{S16}$$

in agreement with known results [103, 104].

The result given by Eq. (S15) is valid for both bithermal and unithermal systems. The algebraic components of the probability density $P$ of velocities at the CL can be examined by expanding the bithermal Boltzmann factor in Eq. (S14) in terms of $\dot{x}_\mathrm{n}$ and $\dot{x}_\mathrm{t}$,

$$P(\dot{x}_\mathrm{n}, \dot{x}_\mathrm{t}) \propto \exp\left[-\left(\frac{m_1\beta_1 n_1^2 + m_2\beta_2 n_2^2}{2\left|\mathbf{M}\right|^2}\dot{x}_\mathrm{n}^2 + \frac{m_1\beta_1 n_2^2 + m_2\beta_2 n_1^2}{2\left|\mathbf{M}\right|^2}\dot{x}_\mathrm{t}^2 - \frac{n_1 n_2 (m_2\beta_2 - m_1\beta_1)}{\left|\mathbf{M}\right|^2}\dot{x}_\mathrm{n}\dot{x}_\mathrm{t}\right)\right]. \tag{S17}$$

It can be seen that for $m_1\beta_1 = m_2\beta_2$ the coupling term disappears and, in this case, the probabilities of each component are separable, i.e, $P = P(\dot{x}_\mathrm{n})P(\dot{x}_\mathrm{t})$. Moreover, for $\dot{x}_\mathrm{t} = 0$, the probability density $P = P(\dot{x}_\mathrm{n})$ is a function of only the normal component. In all other cases the coupling term is nonlinear and the probability densities of each component are not separable. Note that the result derived by Jóhannesson and Jónsson [103] for the expectation value of the normal velocity in a unithermal system with multiple dimensions is in agreement with our result only for unithermal - equimass cases. Away from the equimass limit, discrepancies arise between their result and ours. The nature these discrepancies is that they effectively suppress the coupling term in their calculations by treating $\dot{x}_\mathrm{t} = 0$ only. In our result, we perform a rigorous transformation $(\dot{x}_1, \dot{x}_2) \mapsto (\dot{x}_\mathrm{n}, \dot{x}_\mathrm{t})$ thus including both the coupling term and the tangential component.

## II. GEOMETRICAL ENERGY MINIMUM ACTIVATION ENERGY DERIVATION

At the low-temperature limit, the reaction rate probability will be dominated by the geometrical activation energy (the energy at the well minimum on the CL). To construct this term we want to minimize the energy $E_a$ subject to the crossing condition $E_a = E_b$. As noted by Zwickl *et al.* [98], this optimization can be accomplished using the standard method of Lagrange multipliers with the Lagrange function defined as

$$\mathcal{L} = E_a^{(0)} + \frac{1}{2}k_1(x_1 - \lambda_1)^2 + \frac{1}{2}k_2 x_2^2 + \mu\left(\Delta E_{ba} + \frac{1}{2}k_2\lambda_2^2 - k_2\lambda_2 x_2 - \frac{1}{2}k_1\lambda_1^2 + k_1\lambda_1 x_1\right). \tag{S18}$$

The corresponding system of equations for minimization is

$$\frac{\partial \mathcal{L}}{\partial x_1} = k_1(x_1 - \lambda_1) + \mu k_1 \lambda_1 = 0, \qquad \frac{\partial \mathcal{L}}{\partial x_2} = k_2 x_2 - \mu k_2 \lambda_2 = 0, \tag{S19}$$

and solving this system yields

$$x_1 = (1-\mu)\lambda_1 \quad \text{and} \quad x_2 = \mu\lambda_2. \tag{S20}$$

Substitution into $E_b(x_1, x_2) = E_a(x_1, x_2)$ gives

$$\Delta E_{ba} + \frac{1}{2}k_1\lambda_1^2 + \frac{1}{2}k_2\lambda_2^2 = \mu\left(k_2\lambda_2^2 + k_1\lambda_1^2\right), \tag{S21}$$

in terms of the multiplier $\mu$. The sum of the free energy and reorganization energy can then be expressed as

$$\Delta E_{ba} + E_\mathrm{R} = \mu\left(2E_\mathrm{R}\right). \tag{S22}$$

The multiplier is related to Eq. (S22) through

$$\mu = \frac{\Delta E_{ba} + E_\mathrm{R}}{2E_\mathrm{R}} \quad \text{and} \quad 1 - \mu = -\frac{\Delta E_{ba} - E_\mathrm{R}}{2E_\mathrm{R}}, \tag{S23}$$

from which it follows that the values of the reaction coordinates that allow crossing subject to the constraint are

$$x_1^{\min} = -\lambda_1 \frac{\Delta E_{ba} - E_{\rm R}}{2E_{\rm R}}, \tag{S24}$$

$$x_2^{\min} = \lambda_2 \frac{\Delta E_{ba} + E_{\rm R}}{2E_{\rm R}}. \tag{S25}$$

This point lies on a *line* that connects the metastable minima $E_a(\lambda_1, 0)$ and $E_b(0, \lambda_2)$, and is thus independent of reaction direction [98].

The total activation energy on the $E_a$ surface, $E_{\rm A}^{(a)}$, can be separated into components corresponding to each mode,

$$E_{\rm A}^{(a)} = E_{\rm A1}^{(a)} + E_{\rm A2}^{(a)}, \tag{S26}$$

where A1 and A2 denote activation energy in the respective modes. Following Marcus' theory, ET occurs at the point of minimum energy where $E_a = E_b$. As illustrated through the energy schematic in Fig. 1(c), the activation energy $E_{\rm A}^{(a)}$ is the difference between the occupation energy $E_a^{(0)}$ and the energy at the geometrical equienergetic minimum. In terms of the component energetics the crossing condition gives

$$\begin{aligned} E_{\rm A1}^{(a)} &= \frac{1}{2} k_1 \left( -\lambda_1 \frac{\Delta E_{ba} - E_{\rm R}}{2E_{\rm R}} - \lambda_1 \right)^2 \\ &= E_{\rm R1} \left( \frac{\Delta E_{ba} + E_{\rm R}}{2E_{\rm R}} \right)^2, \end{aligned} \tag{S27}$$

in the $x_1$ coordinate, and

$$\begin{aligned} E_{\rm A2}^{(a)} &= \frac{1}{2} k_2 \lambda_2^2 \left( \frac{\Delta E_{ba} + E_{\rm R}}{2E_{\rm R}} \right)^2 \\ &= E_{\rm R2} \left( \frac{\Delta E_{ba} + E_{\rm R}}{2E_{\rm R}} \right)^2, \end{aligned} \tag{S28}$$

in the $x_2$ coordinate. By combining Eqs. (S26)-(S28), we find the activation energy on the $E_a$ surface at the minimum energy point is

$$E_{\rm A}^{(a)} = \frac{(\Delta E_{ba} + E_{\rm R})^2}{4E_{\rm R}}. \tag{S29}$$

For a unithermal system this activation energy yields the familiar Marcus rate expression [82, 87, 88]. For a bithermal system, the additivity of the total activation energy with respect to its components allows the transfer rate from $a \to b$ to be expressed as

$$\begin{aligned} k_{a\to b} \propto \exp\Bigg[ &-\beta_1 E_{\rm R1} \left( \frac{\Delta E_{ba} + E_{\rm R}}{2E_{\rm R}} \right)^2 \\ &- \beta_2 E_{\rm R2} \left( \frac{\Delta E_{ba} + E_{\rm R}}{2E_{\rm R}} \right)^2 \Bigg] \\ = \exp &\left[ -\Big(\beta_1 E_{\rm R1} + \beta_2 E_{\rm R2}\Big) \left( \frac{\Delta E_{ba} + E_{\rm R}}{2E_{\rm R}} \right)^2 \right]. \end{aligned} \tag{S30}$$

On the $E_b$ surface the activation energy is also a linear combination of components

$$E_{\rm A}^{(b)} = E_{\rm A1}^{(b)} + E_{\rm A2}^{(b)}. \tag{S31}$$

with the $x_1$ component

$$\begin{aligned} E_{\rm A1}^{(b)} &= \frac{1}{2} k_1 \lambda_1^2 \left( \frac{\Delta E_{ba} - E_{\rm R}}{2E_{\rm R}} \right)^2 \\ &= E_{\rm R1} \left( \frac{\Delta E_{ba} - E_{\rm R}}{2E_{\rm R}} \right)^2, \end{aligned} \tag{S32}$$

and the $x_2$ component

$$\begin{aligned} E_{\rm A2}^{(b)} &= \frac{1}{2} k_2 \lambda_2^2 \left( \frac{\Delta E_{ba} + E_{\rm R}}{2E_{\rm R}} - 1 \right)^2 \\ &= E_{\rm R2} \left( \frac{\Delta E_{ba} - E_{\rm R}}{2E_{\rm R}} \right)^2. \end{aligned} \tag{S33}$$

The activation energy on the $E_b$ surface through the minimum energy point is

$$E_{\rm A}^{(b)} = \frac{(-\Delta E_{ba} + E_{\rm R})^2}{4E_{\rm R}}, \tag{S34}$$

and analogous to $k_{a\to b}$ the rate of transfer from surface $E_a$ to surface $E_b$ is

$$k_{b\to a} \propto \exp\left[ -\Big(\beta_1 E_{\rm R1} + \beta_2 E_{\rm R2}\Big) \left( \frac{\Delta E_{ba} - E_{\rm R}}{2E_{\rm R}} \right)^2 \right]. \tag{S35}$$

If $\beta_1 = \beta_2$, then Eqs. (S30) and (S35) give the rate constants derived by Marcus.

## III. RECOVERY OF THE MARCUS RATE EXPRESSIONS

### A. Exact Rate Results

For electron transfer reactions in which donor and acceptor surfaces $E_a$ and $E_b$ are isogeometric ($k_1 = k_2 = k_{\rm M}$) and both modes on each surface are in contact with

baths of the same temperature ($\beta_1 = \beta_2 = \beta$), the bithermal probability densities for each reaction direction:

$$P_{a\to b} = \sqrt{\frac{\beta_1\beta_2(k_1E_{\rm R1}+k_2E_{\rm R2})}{2\pi(\beta_1E_{\rm R2}+\beta_2E_{\rm R1})}} \times \exp\left[-\beta_1\beta_2\frac{(\Delta E_{ba}+E_{\rm R})^2}{4\left(\beta_1E_{\rm R2}+\beta_2E_{\rm R1}\right)}\right], \tag{S36}$$

and

$$P_{b\to a} = \sqrt{\frac{\beta_1\beta_2(k_1E_{\rm R1}+k_2E_{\rm R2})}{2\pi(\beta_1E_{\rm R2}+\beta_2E_{\rm R1})}} \times \exp\left[-\beta_1\beta_2\frac{(\Delta E_{ba}-E_{\rm R})^2}{4\left(\beta_1E_{\rm R2}+\beta_2E_{\rm R1}\right)}\right], \tag{S37}$$

(which are Eqs. (8) and (9)) reduce to

$$P_{a\to b} = \sqrt{\frac{\beta k_{\rm M}}{2\pi}}\exp\left[-\beta\frac{(\Delta E_{ba}+E_{\rm R})^2}{4E_{\rm R}}\right], \tag{S38}$$

and

$$P_{b\to a} = \sqrt{\frac{\beta k_{\rm M}}{2\pi}}\exp\left[-\beta\frac{(\Delta E_{ba}-E_{\rm R})^2}{4E_{\rm R}}\right]. \tag{S39}$$

In the adiabatic limit, the tunneling probability $\mathcal{T}_m \to 1$, and clearly the expectation value $\langle \mathcal{T}_m v_\perp\rangle$ is equal to $\langle v_\perp\rangle$. Moreover, the expression for the velocity term in rate formula given by Eq. (6) is

$$\frac{\langle v_\perp\rangle}{2} = \sqrt{\frac{1}{2\pi m\beta}}, \tag{S40}$$

and, with $\omega_0 = \sqrt{k_{\rm M}/m}$, combining Eqs. (S38) and (S39) with Eq. (S40) gives the expected transition state theory forms

$$k_{a\to b} = \frac{\omega_0}{2\pi}\exp\left[-\beta\frac{(\Delta E_{ba}+E_{\rm R})^2}{4E_{\rm R}}\right], \tag{S41}$$

$$k_{b\to a} = \frac{\omega_0}{2\pi}\exp\left[-\beta\frac{(\Delta E_{ba}-E_{\rm R})^2}{4E_{\rm R}}\right], \tag{S42}$$

in agreement with the adiabatic Marcus rates.

In the nonadiabatic limit, the tunneling probability can calculated using the Landau-Zener expression:

$$\mathcal{T}_m^{\rm LZ} = 1-\exp\left[-\frac{2\pi\Delta^2}{\hbar|\Delta F|_{\alpha_{\rm min}}v_\perp}\right], \tag{S43}$$

where $\Delta$ is the coupling constant between diabatic energy surfaces and $|\Delta F|_{\alpha_{\rm min}}$ is the difference in the forces normal to the CL on each surface evaluated at $\alpha_{\rm min}$ [123, 124]. A first-order approximation to $\mathcal{T}_m^{\rm LZ}$ gives $\mathcal{T}_m \propto 1/v_\perp$ [87]. In this limit, the expectation value $\langle \mathcal{T}_m v_\perp\rangle$ is proportional to a constant and the rate expressions given by combining Eqs. (S38) and (S39) with: Eq. (S40), a first-order approximation to Eq. (S43), and Eq. (6) are

$$k_{a\to b} = \frac{\Delta^2}{\hbar|\Delta F|_{\alpha_{\rm min}}}\sqrt{\frac{\pi\beta k_{\rm M}}{2}}\exp\left[-\beta\frac{(\Delta E_{ba}+E_{\rm R})^2}{4E_{\rm R}}\right], \tag{S44}$$

$$k_{b\to a} = \frac{\Delta^2}{\hbar|\Delta F|_{\alpha_{\rm min}}}\sqrt{\frac{\pi\beta k_{\rm M}}{2}}\exp\left[-\beta\frac{(\Delta E_{ba}-E_{\rm R})^2}{4E_{\rm R}}\right], \tag{S45}$$

which are in agreement with the known nonadiabatic Marcus rates [87, 107].

### B. Approximate Rate Results Using the Tolman Activation Energy

The rate expressions given by Eqs. (35) and (36) can also be applied to recover the Marcus rates. In the Marcus limit ($k_1 = k_2 = k_{\rm M}; \lambda_1 = \lambda_2 = \lambda; \beta_1 = \beta_2 = \beta$), the geometric energy minimum corresponds to the probability maximum, and also corresponds to the activation energy derived by Marcus. We will use this isogeometric-unithermal system to validate the Tolman interpretation of activation energy described in the main text by recovering the Marcus transfer rate. In this case, the total reorganization energy of the system is

$$E_{\rm R} = k_{\rm M}\lambda^2 \tag{S46}$$

and the slope and intercept of the CL are

$$s = 1 \quad \text{and} \quad c = -\frac{\Delta E_{ba}}{k_{\rm M}\lambda}. \tag{S47}$$

Evaluating the expectation value of the activation energy on the CL gives

$$\begin{aligned}\left\langle E_{\rm A}^{(a)}\right\rangle &= \frac{1}{2\beta}+\frac{k_{\rm M}(c-\lambda)^2}{4} \\ &= \frac{1}{2\beta}+\frac{(\Delta E_{ba}+k_{\rm M}\lambda^2)^2}{4k_{\rm M}\lambda^2} \\ &= \frac{1}{2\beta}+\frac{(\Delta E_{ba}+E_{\rm R})^2}{4E_{\rm R}}.\end{aligned} \tag{S48}$$

The corresponding electron transfer rate from site $a$ to site $b$ is

$$k_{a\to b} \propto \exp\left[-\beta\frac{(\Delta E_{ba}+E_{\rm R})^2}{4E_{\rm R}}\right]. \tag{S49}$$

The factor $(\Delta E_{ba}+E_{\rm R})^2/4E_{\rm R}$ is the same as that derived by Marcus. Similarly, the activation energy on the $E_b$

surface is

$$\left\langle E_{\rm A}^{(b)} \right\rangle = \frac{1}{2\beta} + \frac{k_{\rm M}(c+\lambda)^2}{4}$$
$$= \frac{1}{2\beta} + \frac{(-\Delta E_{ba} + k_{\rm M}\lambda^2)^2}{4k_{\rm M}\lambda^2} \quad \text{(S50)}$$
$$= \frac{1}{2\beta} + \frac{(\Delta E_{ba} - E_{\rm R})^2}{4E_{\rm R}},$$

which in turn gives the rate

$$k_{b\to a} \propto \exp\left[-\beta \frac{(\Delta E_{ba} - E_{\rm R})^2}{4E_{\rm R}}\right], \quad \text{(S51)}$$

as expected. Thus, the exponential portions of the rate expressions derived using Eqs. (35) and (36) using the Tolman interpretation of the activation energy are in agreement with the Marcus rates for both the $a \to b$ and $b \to a$ transitions.

## IV. COMPARISON OF RATES

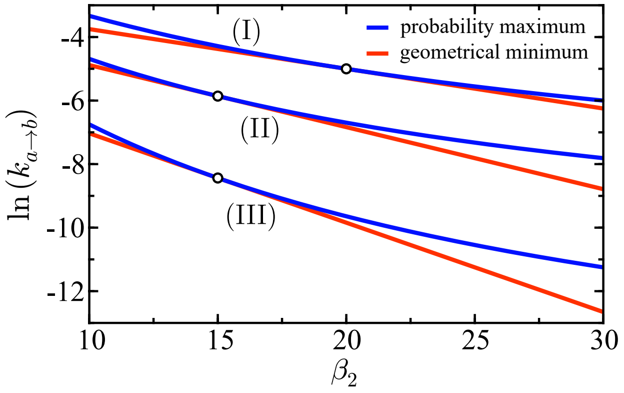


FIG. S1. Electron transfer rate $\ln(k_{a\to b})$ given by the geometrical energy minimum (red) and probablity maximum (blue) shown as function of $\beta_2$ with $\beta_1$ held constant. Parameters are (I) $\Delta E_{ba} = 0, \beta_1 = 20$, (II) $\Delta E_{ba} = 1/4, \beta_1 = 15$, and (III) $\Delta E_{ba} = 1/2, \beta_1 = 15$. The circular markers denote the points where $\beta_1 = \beta_2$. Other parameters are $E_{\rm R1} = E_{\rm R2} = 1/2$. Pre-exponential factors in the rate expressions have been suppressed.

Shown in Fig. S1 is a comparison between the rates for the $a \to b$ transfer process obtained using the geometrical energy minimum and those predicted using the maximum probability points on the CL with pre-exponential factors suppressed. At the unithermal limit, the rates are equivalent as expected from the previous analysis of the CL statistics. For bithermal systems, due to the inclusion of multiple states in the statistical evaluation, the rates are always greater than or equal to the rates predicted using the geometrical minimum. The activation of a larger portion of the reactant population will increase the flow from hot oscillator to the cold oscillator, and the movement of these electrons leads to the rate increase. Temperature-dependent activation energies [125] lead to nonlinearity in the slope of the corresponding Arrhenius plot, which is also observed for the shown bithermal systems. At the unithermal point, the slopes given by the geometrical and thermal activation energies are equal, but for $\beta_1 \neq \beta_2$ the slopes, and hence the activation energies, deviate. These results give credence to the application of the Tolman interpretation [114, 115] to adequately describe activation energy in bithermal systems. Nonlinear Arrhenius plots with both convex and concave curvatures [116, 126] have been interpreted as arising from the redistribution of energy in sets of modes, so it is perhaps not surprising that a thermal gradient between modes leads to nonlinear activation energies.
